# Supplementary material for: Entropic Density Functional Theory: Entropic Inference and the Equilibrium State of Inhomogeneous Fluids
Source: arXiv:2112.09577 source file (2021-12-17)
Supplement: Supplementary file 1 [file appendix.tex]

\chapter{This Is An Appendix}

Here is my appendix content.
